# Supplementary material for: Wasserstein Auto-Encoders of Merge Trees (and Persistence Diagrams)
Source: arXiv:2307.02509 source file (2023-11-09)
Supplement: Supplementary file 1 [file appendixEnergyEvolution.tex]

\section{Energy Evolution}
\begin{figure}
  \centering
  \includegraphics[width=\linewidth]{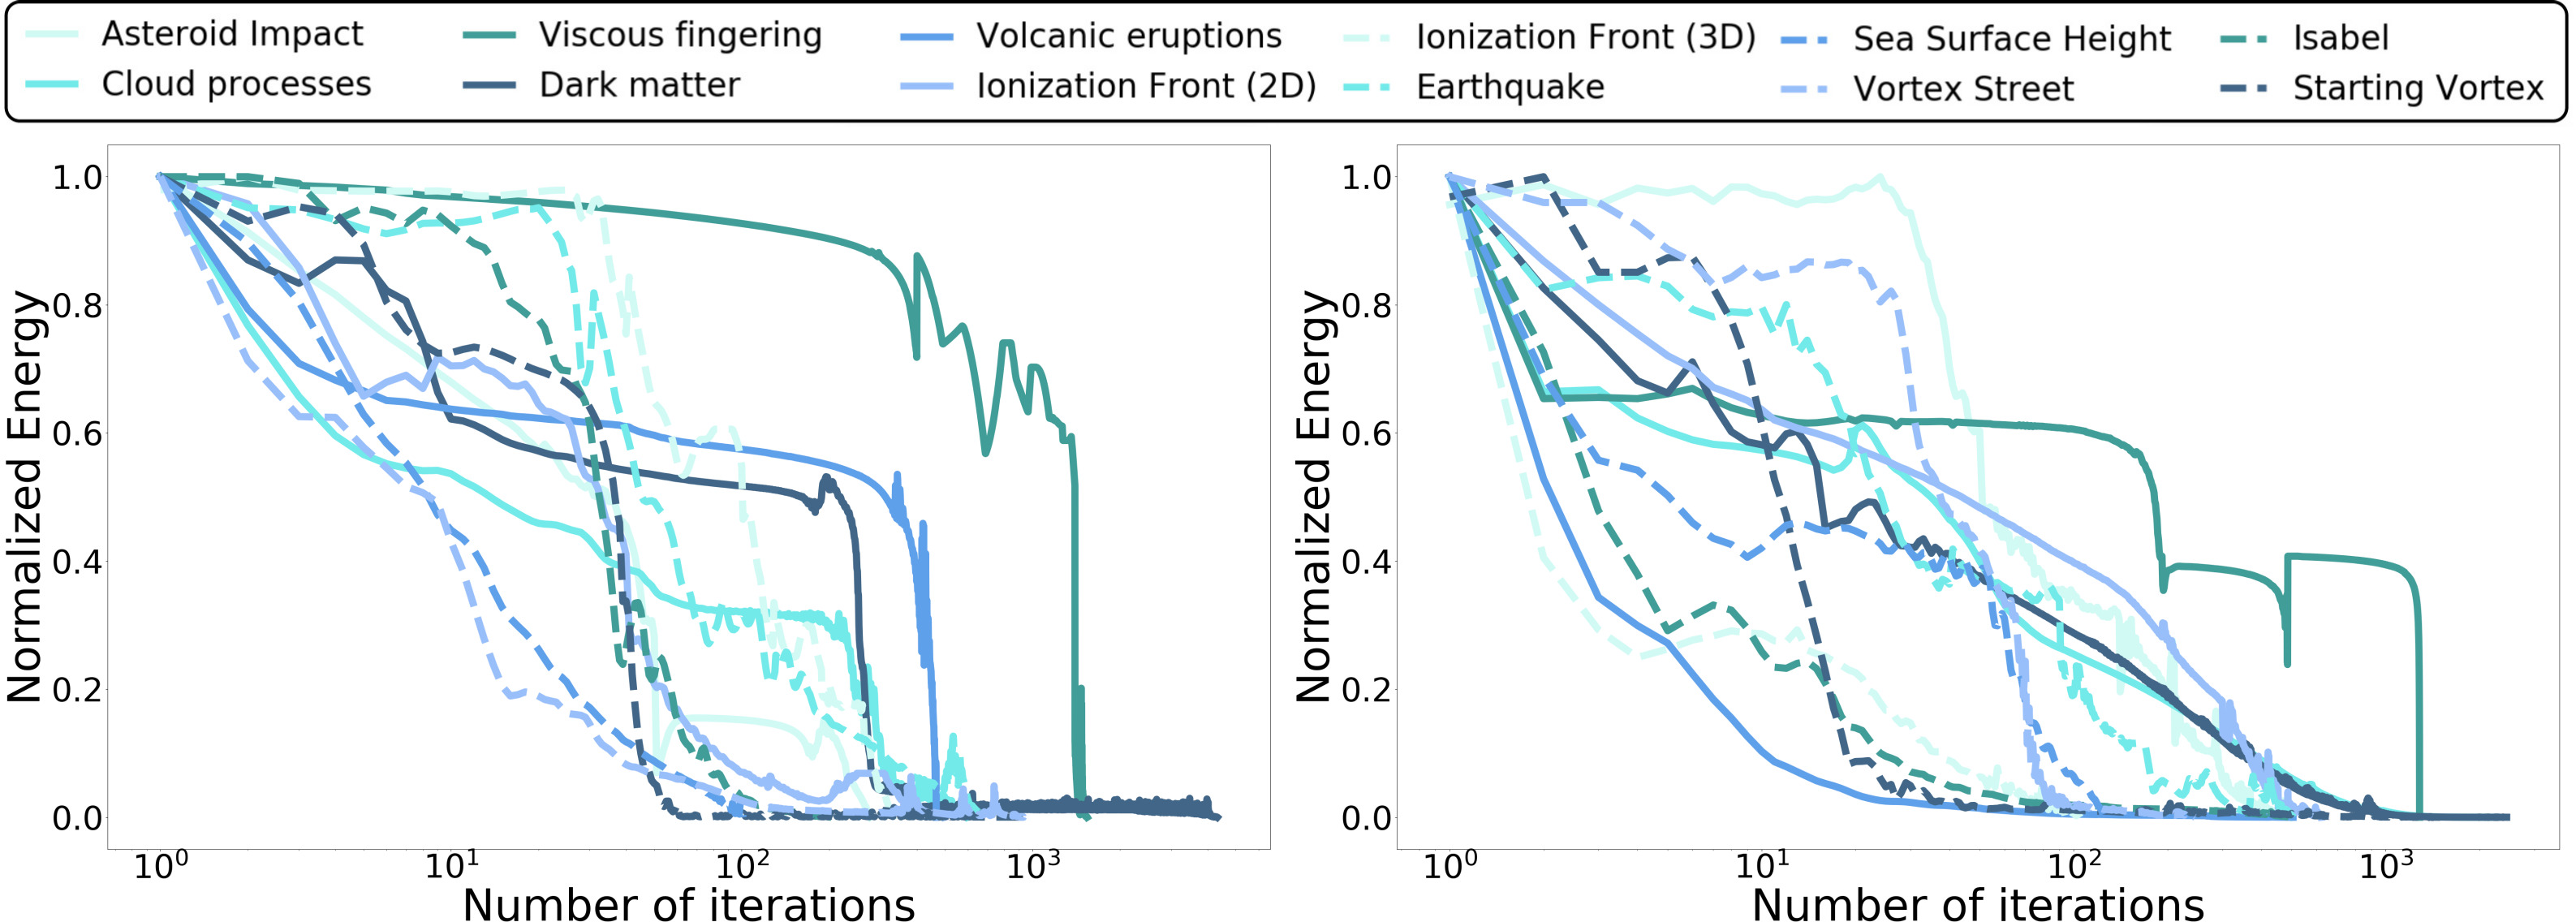}
  \caption{Evolution of the normalized reconstruction error along the
iterations, for PD-WAE (left) and MT-WAE (right).}
  \label{fig_convergenceFigure}
\end{figure}

\autoref{fig_convergenceFigure} reports the evolution of the normalized
reconstruction error for PD and MT-WAE computations, for all our test
ensembles. As often observed when
optimizing neural networks, typical energy oscillations are present in both
cases. However,
\autoref{fig_convergenceFigure} shows that these oscillations do not prevent
the networks to converge (i.e. to reach a state where the energy decreases by
less than $1\%$ between consecutive iterations).
