# Supplementary material for: Wasserstein Auto-Encoders of Merge Trees (and Persistence Diagrams)
Source: arXiv:2307.02509 source file (2023-11-09)
Supplement: Supplementary file 2 [file appendixPGAvsWAE.tex]

\section{PGA vs WAE}

\begin{figure}
  \centering
  \includegraphics[width=\linewidth]{figs/states/PGAvsWAE/PD_PGA_vs_WAE.jpg}
  \caption{PD PGA vs WAE.}
  \label{fig_pd_pga_vs_wae}
\end{figure}
