# Supplementary material for: Wasserstein Auto-Encoders of Merge Trees (and Persistence Diagrams)
Source: arXiv:2307.02509 source file (2023-11-09)
Supplement: Supplementary file 3 [file appendix_VIS.tex]

\documentclass[review,journal]{vgtc}              % review (journal style)
%\documentclass[review,journal,hideappendix]{vgtc} % review (journal style)
%\documentclass[widereview]{vgtc}                  % wide-spaced review
%\documentclass[preprint,journal]{vgtc}            % preprint (journal style)

%% Uncomment one of the lines above depending on where your paper is
%% in the conference process. ``review'' and ``widereview'' are for review
%% submission, ``preprint'' is for pre-publication in an open access repository,
%% and the final version doesn't use a specific qualifier.

%% If you are submitting a paper to a conference for review with a double
%% blind reviewing process, please use one of the ``review'' options and replace the value ``0'' below with your
%% OnlineID. Otherwise, you may safely leave it at ``0''.
\onlineid{1092}

%% In preprint mode you may define your own headline. If not, the default IEEE copyright message will appear in preprint mode.
%\preprinttext{To appear in IEEE Transactions on Visualization and Computer Graphics.}

%% In preprint mode, this adds a link to the version of the paper on IEEEXplore
%% Uncomment this line when you produce a preprint version of the article 
%% after the article receives a DOI for the paper from IEEE
%\ieeedoi{xx.xxxx/TVCG.201x.xxxxxxx}

%% declare the category of your paper, only shown in review mode
\vgtccategory{Research}

%% please declare the paper type of your paper to help reviewers, only shown in review mode
%% choices:
%% * algorithm/technique
%% * application/design study
%% * evaluation
%% * system
%% * theory/model
\vgtcpapertype{Algorithm / Technique}

%% Paper title.
\title{Wasserstein Auto-Encoders of Merge Trees \\(and Persistence Diagrams)\\--\\Appendix}

%% Author ORCID IDs should be specified using \authororcid like below inside
%% of the \author command. ORCID IDs can be registered at https://orcid.org/.
%% Include only the 16-digit dashed ID.
% \iffalse
\author{%
  Mathieu Pont
  and 
  Julien Tierny
}
% \fi

% \iffalse
\authorfooter{
  %% insert punctuation at end of each item
  \item
    Mathieu Pont and Julien Tierny are with the CNRS and Sorbonne University.
    E-mails: \{firstname.lastname\}@sorbonne-universite.fr
}
% \fi

%% Abstract section.
% \abstract{}

%% Keywords that describe your work. Will show as 'Index Terms' in journal
%% please capitalize first letter and insert punctuation after last keyword
% \keywords{Topological data analysis, ensemble data, merge trees, persistence diagrams.}

%% A teaser figure can be included as follows
% \teaser{
%   \centering
%   %\includegraphics[width=\linewidth]{CypressView}
%   \caption{%
%   	% In the Clouds: Vancouver from Cypress Mountain.
%   	% Note that the teaser may not be wider than the abstract block.%
%   	TODO Teaser
%   }
%   \label{fig:teaser}
% }

%% Uncomment below to disable the manuscript note
%\renewcommand{\manuscriptnotetxt}{}

%% Copyright space is enabled by default as required by guidelines.
%% It is disabled by the 'review' option or via the following command:
%\nocopyrightspace

%%%%%%%%%%%%%%%%%%%%%%%%%%%%%%%%%%%%%%%%%%%%%%%%%%%%%%%%%%%%%%%%
%%%%%%%%%%%%%%%%%%%%%% LOAD PACKAGES %%%%%%%%%%%%%%%%%%%%%%%%%%%
%%%%%%%%%%%%%%%%%%%%%%%%%%%%%%%%%%%%%%%%%%%%%%%%%%%%%%%%%%%%%%%%

%% Tell graphicx where to find files for figures when calling \includegraphics.
%% Note that due to the \DeclareGraphicsExtensions{} call it is no longer necessary
%% to provide the the path and extension of a graphics file:
%% \includegraphics{diamondrule} is completely sufficient.
\graphicspath{{figs/}{figures/}{pictures/}{images/}{./}} % where to search for the images

\iffalse
%% Only used in the template examples. You can remove these lines.
\usepackage{tabu}                      % only used for the table example
\usepackage{booktabs}                  % only used for the table example
\usepackage{lipsum}                    % used to generate placeholder text
\usepackage{mwe}                       % used to generate placeholder figures

%% We encourage the use of mathptmx for consistent usage of times font
%% throughout the proceedings. However, if you encounter conflicts
%% with other math-related packages, you may want to disable it.

\usepackage{mathptmx}                  % use matching math font
\fi

% \usepackage{hyperref}
\usepackage{microtype}                 % use micro-typography (slightly more compact, better to read)
\PassOptionsToPackage{warn}{textcomp}  % to address font issues with \textrightarrow
\usepackage{textcomp}                  % use better special symbols
\usepackage{mathptmx}                  % use matching math font
\usepackage{times}                     % we use Times as the main font
         % a nicer typewriter font
\usepackage{cite}                      % needed to automatically sort the references
\usepackage{tabu}                      % only used for the table example
\usepackage{booktabs}                  % only used for the table example

\usepackage{amssymb}
\usepackage{mathtools}
\usepackage{amsmath}                   % for math align env.
\usepackage{color}
\usepackage{mathptmx}
\usepackage{amssymb}
\usepackage{enumitem}
\usepackage{multicol}
\usepackage{anyfontsize}
\usepackage{amsmath}
\usepackage{algorithmic}
\usepackage{algorithm}
\usepackage{letltxmacro}
\usepackage{esvect}
\usepackage{wrapfig}
\usepackage{multicol}
%\usepackage[dvipsnames]{xcolor}
% set the mathcal font back to default, more readable in my opinion (julien)
% \DeclareMathAlphabet{\mathcal}{OMS}{cmsy}{m}{n}
% \DeclareMathOperator*{\argmax}{arg\,max}
% \DeclareMathOperator*{\argmin}{arg\,min}

% \newcommand{\axisNotation}[1]{\vectorNotation{#1}}

% \newcommand{\normalizedTree}{N}

\newcommand{\cutout}[1]{\textcolor{blue}{#1}}
\renewcommand{\cutout}[1]{}

\newlength{\commentindent}
\setlength{\commentindent}{0.6\linewidth}
\makeatletter
\renewcommand{\algorithmiccomment}[1]{\unskip\hfill\makebox[\commentindent][l]{/
/~#1}\par}
\LetLtxMacro{\oldalgorithmic}{\algorithmic}
\renewcommand{\algorithmic}[1][0]{%
  \oldalgorithmic[#1]%
  \renewcommand{\ALC@com}[1]{%
    \ifnum\pdfstrcmp{##1}{default}=0\else\algorithmiccomment{##1}\fi}%
}
\makeatother

\begin{document}

%%%%%%%%%%%%%%%%%%%%%%%%%%%%%%%%%%%%%%%%%%%%%%%%%%%%%%%%%%%%%%%%
%%%%%%%%%%%%%%%%%%%%%% START OF THE PAPER %%%%%%%%%%%%%%%%%%%%%%
%%%%%%%%%%%%%%%%%%%%%%%%%%%%%%%%%%%%%%%%%%%%%%%%%%%%%%%%%%%%%%%%

%% The ``\maketitle'' command must be the first command after the
%% ``\begin{document}'' command. It prepares and prints the title block.
%% the only exception to this rule is the \firstsection command

\maketitle

\input{appendixBody}

%% if specified like this the section will be ommitted in review mode
\iffalse
\acknowledgments{%
  \textbf{For IEEE VIS}, this section may be included in the \textbf{2-page allotment for References, Figure Credits, and Acknowledgments}.
	
	The authors wish to thank A, B, and C.
  This work was supported in part by a grant from XYZ (\# 12345-67890).%
}
\fi

\iffalse
\section*{Acknowledgments}
{\small We thank the reviewers for their careful feedback and suggestions.
This work is partially supported by the European Commission grant
ERC-2019-COG 
\emph{``TORI''} (ref. 863464, 
\url{https://erc-tori.github.io/}).}
\fi

% \cleardoublepage

\newpage

\bibliographystyle{abbrv-doi}

\bibliography{appendix}

%% ^^^^^   FOR IEEE VIS, EVERYTHING HERE MAY BE INCLUDED IN THE    ^^^^^ %%
%% 2-PAGE ALLOTMENT FOR REFERENCES, FIGURE CREDITS, AND ACKNOWLEDGEMENTS %%

% \appendix % You can use the `hideappendix` class option to skip everything after \appendix

\end{document}
